# Supplementary material for: Home, SafeHome: Smart Home Reliability with Visibility and Atomicity
Source: arXiv:2007.12359 source file (2020-07-24)
Supplement: Supplementary file 1 [file appendix.tex]

\begin{appendices}
    \section{Scheduling Policies for Eventual Visibility}
        \label{sec:apndx:EVdesign}
        %\label{sec:appendix:schedulingPoliciesForEV:app}
        
        %\section{Scheduling Policies for Eventual Visibility}
        %\label{sec:EVdesign:app}

        %\ig{For Shegufta/Rui: please fix duplication of labels in this appendix and main (shortened section)} \SBAc{done}

        We now discuss how, for EV, {\name}'s Scheduler (\Figure~\ref{fig:overall-datastructures}) decides where a routine fits into the (eventual) serialization order. The Scheduler is a pluggable component, with minimal requirements that it satisfies all invariants from \Section~\ref{sec:lineage}. We designed and implemented three scheduling policies. %, differing in how they serialize.

        \subsection{First Come First Serve (FCFS) Scheduling}
            Routines are serialized based on their arrival time, i.e., routine ID. When the scheduler schedules a routine $R$, it adds  lock-access entries for all of $R$'s commands to the {\it end} of the corresponding lineages. Post-leases are  allowed in FCFS. However pre-leases are inapplicable because they would violate the FCFS serialization order (\Section~\ref{sec:locks}).
            
            FCFS is attractive if a user expects routines to execute in the order they were initiated. However, this serialization inflexibility results in long lag to start the routine. In contrast, there are many scenarios where  users are willing to accept a completion order different from arrival, e.g., user submits a batch of routines, multiple users submit routines, etc.

        \subsection{Just-in-Time (JiT) scheduling}
    
    	    Just-in-Time (JiT) scheduling is a greedy approach where a routine is started (moved from  wait queue to  lineage) at the {\it earliest time when it is eligible to start.}
    	    
    	    This {\it  eligibility test} for a routine $R$ checks if it will be able to acquire all its locks. That is, for each device accessed by $R$, the device is now either: a) ``Released'', or b) it is both ``Acquired'' {\it and} a pre-lease or post-lease can be availed by $R$. The eligibility test is performed for all routines in the wait queue. The eligibility test is triggered: (i) whenever a new routine arrives (eligibility test only for that routine), or (ii) whenever a lock-access, for some device $D$, is released by some executing routine. In case (ii)  we minimize overhead of traversing the wait queue by running the eligibility test only on those waiting routines  desiring to access device $D$.
    	    
    	    JiT could cause starvation, e.g., a routine $R_{AB}=\{A=ON; B=5;\}$ could be indefinitely starved by periodic invocations of two routines  $R_{A}=\{A=OFF;\}$ and $R_B=\{B=10;\}$. We mitigate starvation by using a TTL (time-to-live) for each routine in the wait-queue (initialized to 5 in \name). The Routine $R$'s TTL is decremented whenever a routine with a higher ID, and accessing a common device with $R$, is scheduled from the wait queue instead of $R$. 
    	    %in the wait queue which accesses a common device with $R$ is scheduled while $R$ is still waiting. 
    	    When its TTL reaches 0, $R$ \textit{must} be scheduled earlier than higher ID routines. % i.e., a newer conflicting routine $R'$ (higher ID) cannot be scheduled earlier. 
    	    If multiple routines with TTL=0 exist, they are scheduled starting from the head of the queue.

    	%%%%%%%%%%%%%%%%%%%%%%%%%%%%%%%%%%%%%%%%%%%%%%%%%%%%%%%%%%%%%%%
    	\subsection{Timeline Scheduling}
    	    \label{sec:timelineScheduling}
    	    
            It may be possible to start some routines even earlier than their eligibility test being satisfied. The Timeline Scheduling policy uses estimates of lock-access durations ($\tau_{R}$), and attempts to place waiting routines into the gaps in the lineage table's timeline (using lock acquisitions, pre-leases, and post-leases). It finds the {\it earliest} possible schedule leveraging existing gaps so as: a) not to violate past/existing serialization order decisions, and b) does not prolong already-running routines beyond an acceptable threshold. This search is triggered for all waiting routines, upon every routine arrival or finish.
    	
    	    \begin{algorithm}
        		\caption{Timeline scheduling of routine $R$}
        		\label{algo:scheduling}
        		\small
        		\begin{algorithmic}[1] % 0 means no line numbering, 1 means number every line
        			
        			\Function{Schedule}{$R$, index, startTime, preSet, postSet}
        			
        			\State devID = $R[index].devID$
        			\State{duration = $lock\_access(R, devID).duration$}\label{line:duration}
        
        			\State{//return from recursion}
        			\If{{\tt $R.cmdCount$ < index}}
        			    \State{\Return true} \label{line:baseCase}
        			\EndIf 
        						
        			\State{//Find gap and pre- and post-set}
        			\State gap = getGap(devID , startTime, duration) \label{line:gap}
        			\State curPreSet = preSet $\cup$ getPreSet(lineage[devID], gap.id) 
        			\State curPostSet = postSet $\cup$ getPostSet(lineage[devID], gap.id)
        			
            		\If{{\tt curPreSet $\cap$ curPostSet = $\emptyset$} } \label{line:intersection}
            			\State{//Serialization is not violated}
            			
            			\State canSchedule = schedule($R$, index + 1, gap.startTime + duration , curPreSet, curPostSet) \label{line:deepDiveCall}
            			
            			\If{{\tt canSchedule}}
                			\State { lineage[devID].insert($R[index]$, gap)}
                			\State {\Return true}
            			\EndIf
        			\EndIf			
        			\State {//backtrack: try next gap}
        			\State{\Return {schedule($R$, index, gap.startTime + duration , preSet, postSet)} \label{line:backtrack}}
        			\EndFunction
        			
        		\end{algorithmic}
        	\end{algorithm}

        	\Algorithm~\ref{algo:scheduling} shows pseudocode. The key idea is to employ a recursive back-tracking strategy trying different gaps. We explain the algorithm by using the  example in 
        	\Figure~\ref{fig:timelineBasedApproach}. \Figure~\ref{fig:timelineBasedApproach_a} depicts a lock table right before routine $R_3=\{C \rightarrow B\}$ arrives at time $T_{R3}$, and has four gaps in the lineage. 
        	Starting with the first device in the routine ($C$ for $R_3$):  $\tau_{R_3}(C)$ (\Line~\ref{line:duration}), the Timeline scheduler finds the first gap in $C$'s lineage that can fit $\tau_{R_3}(C)$ (\Line~\ref{line:gap}). This is Gap 1 in \Figure~\ref{fig:timelineBasedApproach_a}.

    	    Next, the Timeline scheduler validates that this gap choice will not violate previously decided serializations. For the scheduled lock-accesses of $R_3$ so far, it builds two sets: a) \textit{preSet:} the union of all (executing and scheduled) routines  placed \textit{before} $R_3$'s lock-accesses ($\{R_1\}$ in \Figure~\ref{fig:timelineBasedApproach_b}), and b) \textit{postSet:} the union of all (executing and scheduled) routines placed \textit{after} $R_3$'s lock-accesses ($\{R_1, R_2\}$ in \Figure~\ref{fig:timelineBasedApproach_b}). The preSet and postSet of $R$ represent the routines positioned before and after $R$,  respectively, in the serialization order. {\it The gap choice is valid if and only if the  intersection of the preSet and the postSet is empty.} In this case, the scheduler moves on to the next command of the routine. Otherwise (e.g., as in \Figure~\ref{fig:timelineBasedApproach_b}), the scheduler backtracks and tries the next gap (\Line~\ref{line:backtrack}). This process then repeats.

\end{appendices}
